# Supplementary material for: Brownian asymmetric simple exclusion process
Source: arXiv:1807.00138 ancillary file (2018-09-01)
Supplement: Supplementary file 1 [file Lips_etal_arXiv_Supplemental_Material.pdf]

# Supplemental Material
# Brownian asymmetric simple exclusion process (BASEP)

Dominik Lips, Artem Ryabov, and Philipp Maass

## 1. Evolution equation for the particle density

Here we derive the exact evolution equation for the particle density by considering the stochastic many-particle dynamics in an "extended zone scheme". Readers not interested in details of this derivation, may start with the analysis below in the second section of this supplemental material.

For Langevin equations as in Eq. (1) of the main text, the Smulochowski equation describes the time evolution of the joint probability density $w_N = w_N(y_1, \ldots, y_N, t)$ of finding the $N$ particles at positions $y_1, \ldots, y_N$ at time $t$:

$$\frac{\partial w_N}{\partial t} = -\sum_{i=1}^{N} \frac{\partial j_i}{\partial y_i}\,, \tag{S1a}$$

$$j_i = j_i(y_1, \ldots, y_N, t) = \mu\,[f^{\rm ext}(y_i) + f_i^{\rm int}(y_1, \ldots y_N)]\, w_N - D\frac{\partial w_N}{\partial y_i}\,. \tag{S1b}$$

In the case of a one-dimensional motion of particles that can not pass each other, we assume an ordering $y_1 < \ldots < y_N$ of their positions. If interaction forces are present solely between nearest neighboring particles, periodic boundary conditions can be dealt with by assuming the initial particles positions $y_i(0)$ at time $t = 0$ to lie in the interval $[0, L[$ and by imagining two mirrors of the last ($i = N$) and first particle ($i = 1$) with indices 0 and $(N + 1)$ to be added to the system, respectively. These mirror particles have enslaved coordinates

$$y_0 = y_N - L\,, \tag{S2a}$$

$$y_{N+1} = y_1 + L\,, \tag{S2b}$$

for all times $t > 0$. The probability density $w_N(y_1, \ldots, y_N, t)$ then describes the dynamics in the "extended zone scheme" with $y_i \in \mathbb{R}$ and $w_N(y_1, \ldots, y_N, t) = 0$ for $(y_N - y_1) \geq L$. This holds because the particles $i = 1$ and $i = N$ cannot pass the mirror particles $i = 0$ and $i = N + 1$, respectively.

For connecting $w_N(y_1, \ldots, y_N, t)$ to the probability density of finding the particles at positions

$$x_i = y_i \bmod L\,, \quad i = 1, \ldots, N\,, \tag{S3}$$

on a ring of size $L$, i.e. in the "reduced zone scheme" with $x_i \in [0, L[$, we need to take into account the number of circulations of the particles along the ring until time $t$. In a system without (continuous) translational invariance in space, it is convenient to set $x_i(0) = y_i(0)$, $i = 1, \ldots, N$, for the starting positions and to introduce a net winding number

$$n(t) = \mathrm{int}(y_1(t)/L)\,, \tag{S4}$$

where $\mathrm{int}(x) \in \mathbb{Z}$ is the integer part of $x \in \mathbb{R}$. This net winding number gives for the particle $i = 1$ the number of passages of the point $x = 0$ in clockwise direction minus the number of passages in counterclockwise direction until time $t$. Given $n$ and a particle configuration $(x_1, \ldots, x_N)$ at any time $t \geq 0$, the corresponding net winding numbers $n_i$ of all particles (including the first) are

$$n_i = n + \begin{cases} 1\,, & x_i < x_1\,, \\ 0\,, & x_i \geq x_1\,, \end{cases} \quad i = 1, \ldots, N\,. \tag{S5}$$

Accordingly, we obtain for the respective particle positions in the extended zone scheme

$$y_i = x_i + n_i L\,, \quad i = 1, \ldots, N\,, \tag{S6}$$

with the $n_i$ given by Eq. (S4). Note that $y_1 < \ldots < y_N$ and $(y_N - y_1) < L$. The joint probability density $p_N(x_1, \ldots, x_N, n, t)$ of finding, at time $t$, the particles at positions $x_1, \ldots, x_N$ and the winding number to be $n$, is thus connected to $w_N(y_1, \ldots, y_N, t)$ by

$$p_N(x_1, \ldots, x_N, n, t) = w_N(x_1 + n_1 L, \ldots, x_N + n_N L, t)\,. \tag{S7a}$$

Introducing the marginal probability density

$$w_1(y,t)=\int_{-\infty}^{\infty}\mathrm{d}y_2\ldots\int_{-\infty}^{\infty}\mathrm{d}y_N\,w_N(y,y_2,\ldots,y_N,t)\,,\tag{S8}$$

we can express the probability density $p_1(x,t)$ of finding the particle $i=1$ at ring position $x$ at time $t$ as

$$p_1(x,t)=\sum_{n=-\infty}^{\infty}w_1(x+nL,t)\,.\tag{S9}$$

For particles of size $\sigma$ with hard-core interactions, we have $f_i^{\mathrm{int}}=0$ in Eq. (S1), but need to take into account the constraints $(y_{i+1}-y_i)\geq\sigma$ for $i=0,\ldots,N$. This means that the configuration space is restricted and integrals over successive particle coordinates can be written as

$$\int\mathrm{d}y_i\int\mathrm{d}y_{i+1}\ldots\int\mathrm{d}y_k\ldots=\int\mathrm{d}y_i\ldots\int\mathrm{d}y_k\prod_{l=i-1}^{k}\theta(y_{l+1}-y_l-\sigma)\ldots\,,\tag{S10}$$

where $\theta(x)$ is the Heaviside step function [$\theta(x)=1$ for $x\geq 0$ and zero otherwise]. Moreover, because at contact of the particles $i$ and $(i+1)$ the currents $j_i$ and $j_{i+1}$ must be equal, it holds

$$\Big[j_i(y_1,\ldots,y_N,t)-j_{i+1}(y_1,\ldots,y_N,t)\Big]_{y_{i+1}=y_i+\sigma}=0\,,\quad i=0,\ldots,N\,.\tag{S11}$$

These equations constitute boundary conditions for the Smoluchowski equation (S1), where $j_0=j_N$ and $j_{N+1}=j_1$.

Integrating the Smoluchowski equation over the coordinates $y_2,\ldots,y_N$, one obtains, after some algebra under consideration of the boundary equations,

$$\frac{\partial w_1(y_1,t)}{\partial t}=-\frac{\partial}{\partial y_1}\int\mathrm{d}y_2\ldots\int\mathrm{d}y_N\prod_{i=1}^{N}\theta(y_{i+1}-y_i-\sigma)j_1(y_1,y_2,\ldots,y_N,t)\,.\tag{S12}$$

Inserting $j_1(y_1,y_2,\ldots,y_N,t)$ from Eq. (S1b) yields

$$\begin{aligned}\frac{\partial w_1(y_1,t)}{\partial t}&=-\frac{\partial}{\partial y_1}\left[\mu f^{\mathrm{ext}}(y_1)w_1(y_1,t)-D\int\mathrm{d}y_2\ldots\int\mathrm{d}y_N\prod_{i=1}^{N}\theta(y_{i+1}-y_i-\sigma)\frac{\partial}{\partial y_1}w_N(y_1,\ldots,y_N,t)\right]\\&=-\frac{\partial}{\partial y_1}\left[\mu f^{\mathrm{ext}}(y_1)w_1(y_1,t)-D\,\frac{\partial w_1(y_1,t)}{\partial y_1}\right.\\&\qquad\left.+D\int\mathrm{d}y_2\ldots\int\mathrm{d}y_N\,w_N(y_1,\ldots,y_N,t)\frac{\partial}{\partial y_1}\prod_{i=1}^{N}\theta(y_{i+1}-y_i-\sigma)\right].\end{aligned}\tag{S13}$$

With $y_{N+1}=y_1+L$ from Eq. (S2b) it holds

$$\begin{aligned}\frac{\partial}{\partial y_1}\prod_{i=1}^{N}\theta(y_{i+1}-y_i-\sigma)&=-\delta(y_2-y_1-\sigma)\prod_{i=2}^{N}\theta(y_{i+1}-y_i-\sigma)+\delta(y_1+L-y_N-\sigma)\prod_{i=1}^{N-1}\theta(y_{i+1}-y_i-\sigma)\\&=\prod_{i=1}^{N}\theta(y_{i+1}-y_i-\sigma)\left[\delta(y_N-y_1-L+\sigma)-\delta(y_2-y_1-\sigma)\right]\,.\end{aligned}\tag{S14}$$

The integral in the last term of Eq. (S13) therefore gives

$$\begin{aligned}&\int\mathrm{d}y_2\ldots\int\mathrm{d}y_N\,w_N(y_1,\ldots,y_N,t)\frac{\partial}{\partial y_1}\prod_{i=1}^{N}\theta(y_{i+1}-y_i-\sigma)\\&\quad=\int\mathrm{d}y_1'\ldots\int\mathrm{d}y_N'\prod_{i=1}^{N}\theta(y_{i+1}'-y_i'-\sigma)\,w_N(y_1',\ldots,y_N',t)\delta(y_1'-y_1)\left[\delta(y_N'-y_1-L+\sigma)-\delta(y_2'-y_1-\sigma)\right]\\&\quad=\Psi_{1N}(y_1,y_1+L-\sigma,t)-\Psi_{12}(y_1,y_1+\sigma,t)\,,\end{aligned}\tag{S15}$$

where $\Psi_{jk}(y,z,t)$ denotes the joint probability of finding particles $j$ and $k$ at positions $y$ and $z$ at time $t$, respectively. Inserting this in Eq. (S13) yields, using $D=\mu k_{\rm B}T$,

$$\frac{\partial w_1(y,t)}{\partial t}=-\frac{\partial}{\partial y}\left(\mu f^{\rm ext}(y)w_1(y,t)+\mu k_{\rm B}T\left[\Psi_{1N}(y,y+L-\sigma,t)-\Psi_{12}(y,y+\sigma,t)\right]-D\,\frac{\partial w_1(y,t)}{\partial y}\right). \tag{S16}$$

An analogous equation holds for each marginal density $w_i(y,t)$, $i=2,...,N$, of the other $(N-1)$ particles, if $\Psi_{1N}=\Psi_{10}$ and $\Psi_{12}$ are replaced by $\Psi_{i,i-1}$ and $\Psi_{i,i+1}$ $[\Psi_{N,N+1}=\Psi_{N,1}]$. As in Eq. (S9), $p_i(x,t)=\sum_{n=-\infty}^{\infty}w_i(x+nL,t)$ gives the probability density of finding the $i$th particle at ring position $x$ at time $t$. For the local particle density $\rho_{\rm loc}(x,t)=\sum_{i=1}^{N}p_i(x,t)$ on the ring, i.e. the probability of finding any of the $N$ particles at ring position $x$ at time $t$, we then obtain

$$\begin{aligned}\frac{\partial\rho_{\rm loc}(x,t)}{\partial t}&=\sum_{i=1}^{N}\frac{\partial p_i(x,t)}{\partial t}=\sum_{i=1}^{N}\sum_{n=-\infty}^{\infty}\frac{\partial w_i(x+nL,t)}{\partial t}\\&=-\frac{\partial}{\partial x}\left(\mu f^{\rm ext}(x)\rho_{\rm loc}(x,t)+\mu k_{\rm B}T\left[\Psi_-(x,t)-\Psi_+(x,t)\right]-D\,\frac{\partial\rho_{\rm loc}(x,t)}{\partial x}\right).\end{aligned} \tag{S17}$$

Here we have used the $\lambda$-periodicity (and consequently $L$-periodicity) of $f^{\rm ext}(y)$ and introduced the joint probabilities $\Psi_-(x,t)=\sum_{i=1}^{N}\sum_{n=-\infty}^{\infty}\Psi_{i,i-1}(x+nL,x+(n+1)L-\sigma,t)$ and $\Psi_+(x,t)=\sum_{i=1}^{N}\sum_{n=-\infty}^{\infty}\Psi_{i,i+1}(x+nL,x+nL+\sigma,t)$ of finding a particle at ring position $x$ and a neighboring particle in contact (at distance $\sigma$) to it in counterclockwise and clockwise direction at time $t$, respectively. With $\psi_\pm(x,t)=\Psi_\pm(x,t)/\rho_{\rm loc}(x,t)$ we denote the respective conditional probabilities. According to Eq. (S17), the hard-core interaction mediated by the neighbors of a particle at position $x$ thus gives rise to mean contact forces $\mp k_{\rm B}T\psi_\pm(x,t)$. These add to a mean interaction force

$$\langle f^{\rm int}(x,t)\rangle=\frac{k_{\rm B}T}{\rho_{\rm loc}(x,t)}\left[\Psi_-(x,t)-\Psi_+(x,t)\right]=k_{\rm B}T\left[\psi_-(x,t)-\psi_+(x,t)\right]. \tag{S18}$$

In fact, an analogous calculation for particles allowed to pass each other and interacting via (sufficiently short-ranged) pair forces $f^{(2)}(y_i,y_k)$, i.e. $f_i^{\rm int}(y_1,\ldots y_N)=\sum_{k,k\neq i}f^{(2)}(y_i,y_k)$ in Eq. (S1), also yields Eq. (S17), but with $k_{\rm B}T[\Psi_-(x,t)-\Psi_+(x,t)]$ replaced by $\int dy\rho_2(x,y,t)\,f^{(2)}(x,y)=\langle f^{\rm int}(x,t)\rangle\rho_{\rm loc}(x,t)$, where $\rho_2(x,y,t)=\sum_{i\neq k}\langle\delta(y_i(t)-x)\delta(y_k(t)-y)\rangle$ is the two-particle density. This gives back Eq. (S17) if setting $f^{(2)}(x,y)=k_{\rm B}T[\delta(y-x+\sigma)-\delta(y-x-\sigma)]$ and taking into account the hard-core constraint. The latter implies that only $N$ of the $N(N-1)$ $\delta$-function terms in $\rho_2(x,y,t)$ contribute to $\langle f^{\rm int}(x,t)\rangle$. These $N$ terms correspond to the possibilities of occupying the position $x$ with any of the particles.

### 2. Current in the non-equilibrium steady state

In the non-equilibrium steady state (NESS), we obtain from Eqs. (S17) and (S18) the constant particle current (or, more precisely, current density)

$$j=\mu[f^{\rm ext}(x)+\langle f^{\rm int}(x)\rangle]\rho_{\rm loc}(x)-D\,\frac{{\rm d}\rho_{\rm loc}(x)}{{\rm d}x}=\mu\left[f-\frac{{\rm d}U(x)}{{\rm d}x}+\langle f^{\rm int}(x)\rangle\right]\rho_{\rm loc}(x)-D\,\frac{{\rm d}\rho_{\rm loc}(x)}{{\rm d}x}. \tag{S19}$$

Because the external potential $U(x)$ is a $\lambda$-periodic function, both the number density $\rho_{\rm loc}(x)$ and the mean interaction force $\langle f^{\rm int}(x)\rangle$ in the NESS must be $\lambda$-periodic as well. Dividing Eq. (S19) by $\rho_{\rm loc}(x)$ and integrating thereafter over $x$ from 0 to $\lambda$ thus yields

$$j=\frac{\mu\left[f\lambda+\int_0^\lambda{\rm d}x\langle f^{\rm int}(x)\rangle\right]}{\displaystyle\int_0^\lambda\frac{{\rm d}x}{\rho_{\rm loc}(x)}}=\frac{\mu\left[f+\bar f^{\rm int}\right]}{\displaystyle\frac{1}{\lambda}\int_0^\lambda\frac{{\rm d}x}{\rho_{\rm loc}(x)}}, \tag{S20}$$

where $\bar f^{\rm int}=\int_0^\lambda{\rm d}x\langle f^{\rm int}(x)\rangle/\lambda$ is the period-averaged mean interaction force in the NESS. The joint probabilities $\Psi_\pm(x)$ are also $\lambda$-periodic in the NESS. For $\sigma=\lambda$, it moreover holds $\Psi_-(x)=\Psi_+(x)$ and all $x$, and hence $\langle f^{\rm int}(x)\rangle=0$ according to Eq. (S18). Likewise, $\langle f^{\rm int}(x)\rangle=0$ for point particles with $\sigma=0$.

Hence, for $\sigma=0,\lambda$, Eq. (S19) becomes the same as for non-interacting particles and gives an inhomogeneous linear differential equation of first order for $\rho_{\rm loc}(x)$. Considering the periodic boundary condition $\rho_{\rm loc}(0)=\rho_{\rm loc}(\lambda)$ and the

normalization condition $\int_0^\lambda \mathrm{d}x \rho_{\mathrm{loc}}(x)/\lambda = \rho$, one obtains the solutions $\rho_{\mathrm{loc}}(x) = \rho_{\mathrm{loc}}^{(0)}(x)$ and $j = j_0$ with [1]:

$$\rho_{\mathrm{loc}}^{(0)}(x) = \rho \, \frac{g(x)\left[\dfrac{G(\lambda)}{1-e^{-\beta f\lambda}} - G(x)\right]}{\displaystyle\int_0^\lambda \frac{\mathrm{d}x}{\lambda} g(x)\left[\dfrac{G(\lambda)}{1-e^{-\beta f\lambda}} - G(x)\right]}\,, \tag{S21a}$$

$$j_0 = \frac{\mu f}{\displaystyle\frac{1}{\lambda}\int_0^\lambda \frac{\mathrm{d}x}{\rho_{\mathrm{loc}}^{(0)}(x)}} = \frac{D\rho}{\lambda}\,\frac{1}{\displaystyle\int_0^\lambda \frac{\mathrm{d}x}{\lambda} g(x)\left[\dfrac{G(\lambda)}{1-e^{-\beta f\lambda}} - G(x)\right]} = v_0\rho\,, \tag{S21b}$$

where $v_0$ is the mean velocity of a single particle,

$$g(x) = \exp\left(\beta f\lambda - \beta[U(x) - U(0)]\right) = g(x+\lambda)\,, \tag{S21c}$$

$$G(x) = \int_0^x \frac{\mathrm{d}x'}{\lambda}\frac{1}{g(x')}\,, \tag{S21d}$$

and $\beta = 1/(k_{\mathrm{B}}T)$. For $\sigma \neq 0, \lambda$ in contrast, $\bar{f}^{\mathrm{int}}$ in general contributes to the current and depends on the density profile $\rho_{\mathrm{loc}}(x)$ and density correlations $\Psi_\pm(x)$.

**3. Linear response behavior of the current**

In equilibrium ($f = 0$), it must hold $\bar{f}^{\mathrm{int}} = 0$ and $\langle f^{\mathrm{int}}(x)\rangle$ will be an antisymmetric function with respect to the points of local minima (or maxima) of $U(x)$. Close to equilibrium, in the linear response limit, we obtain from Eq. (S20)

$$j = \frac{\mu(1+\alpha)f}{\displaystyle\frac{1}{\lambda}\int_0^\lambda \frac{\mathrm{d}x}{\rho_{\mathrm{eq}}(x)}}\,, \quad \alpha = \left.\frac{\partial \bar{f}^{\mathrm{int}}}{\partial f}\right|_{f=0}\,, \tag{S22}$$

where $\rho_{\mathrm{eq}}(x)$ is the number density in equilibrium. We can interpret this formula by saying that the interaction renormalizes the bare mobility $\mu$ to $\tilde{\mu} = (\mu + \alpha)$ and that $[\mu\rho_{\mathrm{eq}}(x)]^{-1}(\mathrm{d}x/\lambda)$ gives the resistivities of line segments $\mathrm{d}x$ and the integral over them the total resistivity or inverse conductivity.

The number density in equilibrium can be obtained by minimizing the (in the grand-canonical ensemble) exact density functional $\Omega[\rho]$ of hard rods in one dimension [2],

$$\Omega[\rho(x)] = \int_0^\lambda \mathrm{d}x \rho(x)\left\{U - \mu_{\mathrm{chem}} - k_{\mathrm{B}}T\left[1 - \log\left(\frac{\rho(x)}{1-\int_{x-\sigma}^x \mathrm{d}y\,\rho(y)}\right)\right]\right\}\,, \tag{S23}$$

where the chemical potential $\mu_{\mathrm{chem}}$ is fixed by $\rho = \int_0^\lambda \mathrm{d}x\rho_{\mathrm{eq}}(x)/\lambda$. The condition $\delta\Omega/\delta\rho(x) = 0$ yields the structure equation [relation between $\rho_{\mathrm{eq}}(x)$ und $U(x)$]

$$\rho_{\mathrm{eq}}(x) = \exp\left(-\beta[U(x) - \mu_{\mathrm{chem}}]\right)\left(1 - \int_{x-\sigma}^x \mathrm{d}y\,\rho_{\mathrm{eq}}(y)\right)\exp\left(-\beta\int_x^{x+\sigma}\mathrm{d}z\,\frac{\rho_{\mathrm{eq}}(z)}{1-\int_{x-\sigma}^x \mathrm{d}y\,\rho_{\mathrm{eq}}(y)}\right)\,. \tag{S24}$$

In Eqs. (S23) and (S24), $\rho_{\mathrm{eq}}(x)$ for arguments $x$ outside $[0,\lambda[$ is given by the $\lambda$-periodicity of $\rho_{\mathrm{eq}}(x)$. For $\sigma = 0$, the integrals over $\rho_{\mathrm{eq}}(x)$ in Eq. (S24) are zero and $\rho_{\mathrm{eq}}(x) = \exp(-\beta[U(x) - \mu_{\mathrm{chem}}])$ as for non-interacting particles. For $\sigma = \lambda$, the terms in Eq. (S24) containing the integrals give the constant $(1-\rho\lambda)\exp[-\beta\rho\lambda/(1-\rho\lambda)]$, i.e. one obtains the same equilibrium density as for non-interacting particles (and a modified chemical potential). Hence, taking into account $\bar{f}^{\mathrm{int}} = 0$ for $\sigma = 0, \lambda$ as discussed above, Eq. (S20) reduces to the linear-response current of independent particles [1].

To analyze $j = j(\rho,\sigma)$ for $\sigma \neq 0, \lambda$ in the linear response limit, a simple approximation is to neglect the contribution from $\bar{f}^{\mathrm{int}}$, i.e. to set $\alpha = 0$ in Eq. (S22). This corresponds to a result that was obtained also when making a Hartree ansatz for solving the Smolchowski equation [3, 4]. We carried out a calculation for $\alpha = 0$, where we determined $\rho_{\mathrm{eq}}(x)$ by minimizing $\Omega[\rho(x)]$ from Eq. (S23). The results for $j = j(\rho,\sigma)$ are shown in Figs. S1(a) and S1(b) in correspondence to Figs. 2(a) and 2(b) in the main text. As can be seen from these figures, the behavior resulting from the interplay of the barrier reduction, blocking and exchange symmetry effect, as discussed in the main text, is

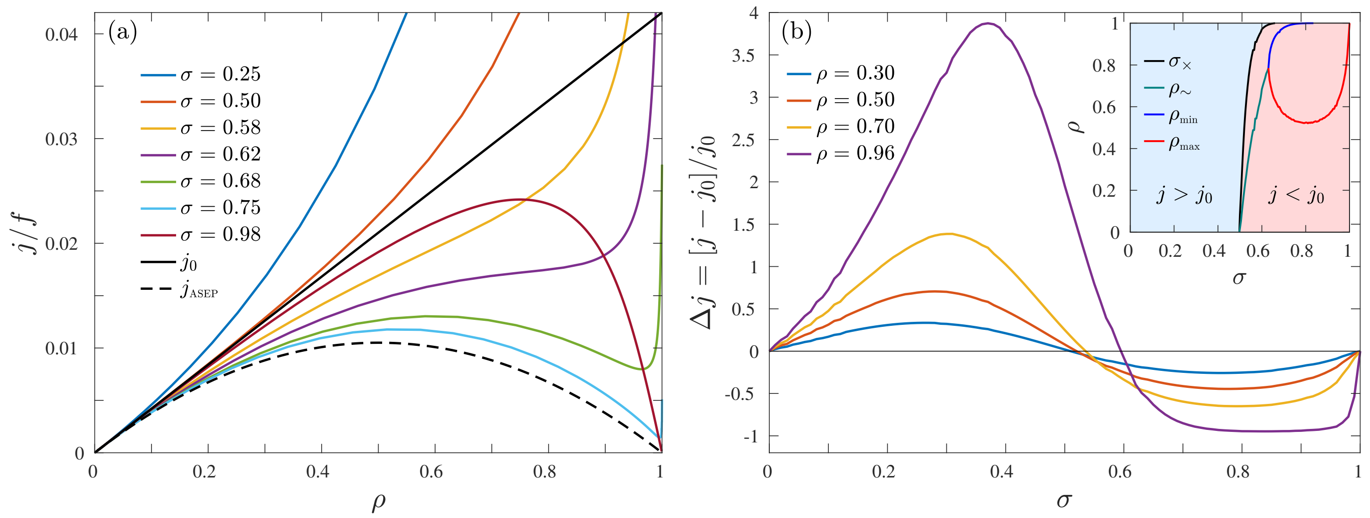


FIG. S1. Approximate linear response results for the current in the BASEP when setting $\alpha = 0$ in Eq. (S22) and determining $\rho_{\text{eq}}(x)$ from Eq. (S23). The plots correspond to Figs. 2(a) and 2(b) of the main text: In (a) $j(\rho,\sigma)$ is plotted as a function of $\rho$ for various fixed particle sizes $\sigma$. The solid and dashed black lines mark the currents $j_0(\rho)$ and $j_{\text{ASEP}}(\rho)$ for non-interacting particles and the corresponding ASEP, respectively. In (b) the current change $\Delta j(\rho,\sigma) = [j(\rho,\sigma)-j_0(\rho)]/j_0(\rho)$ due to hard-core interactions is shown for different fixed densities $\rho$. The inset shows $\sigma_\times(\rho)$, and the dependencies of $\rho_\sim$, $\rho_{\max}$, and $\rho_{\min}$ on $\sigma$.

qualitatively reproduced. This shows that in the linear response limit, these effects are to a large extent mediated via $\rho_{\text{eq}}(x)$ in Eq. (S22).

The analytical calculation of $j(\rho,\sigma)$ can be improved by using dynamical density functional theory [5, 6], which amounts of employing the exact dependence of the pair densities on the densities in an equilibrium system as an approximation for the NESS. The corresponding calculations and results will be presented elsewhere [7].

### 4. Current relation in Eq. (2): Proof and implications

To prove Eq. (2), where $m = \text{int}(\sigma/\lambda)$, we consider the constrained Langevin dynamics in the extended zone scheme,

$$\dot{y}_i = \mu[f + f^{\text{ext}}(y_i)] + \sqrt{2D}\,\eta_i(t)\,, \quad i = 1,\ldots,N\,, \tag{S25}$$

with $y_1 < y_2 < \ldots < y_N$ and the two additional virtual particles having enslaved coordinates $y_0 = y_N - L$, $y_{N+1} = y_1 + L$, [see Eqs. (S2b)(a),(b)], and the constraints $y_{i+1} - y_i \geq \sigma$ for $i = 0,\ldots,N$. Because of the $\lambda$-periodicity of $f^{\text{ext}}(y)$, the transformed coordinates

$$y'_i = y_i - im\lambda\,, \quad i = 0,\ldots,N+1\,, \tag{S26}$$

satisfy the same Langevin equations (S25), but with the modified constraints $y'_{i+1} - y'_i \geq \sigma' = \sigma - m\lambda$ for $i = 0,\ldots,N$. By the transformation the length $L$ gets reduced to $L' = y'_{N+1} - y'_1 = y'_N - y'_0 = L - Nm\lambda$, and the number of periods $M = L/\lambda$ to $M' = L'/\lambda = M - Nm$. Accordingly, the system with the transformed coordinates corresponds to a system of $N' = N$ particles with diameter $\sigma' = \sigma - m\lambda$ and filling factor $\rho' = N'/M' = N/(M - Nm) = \rho/(1 - m\rho)$. Note that $\rho \leq (\lambda/\sigma) \leq (1/m)$ for $\sigma \geq m\lambda$, i.e. $\sigma - m\lambda$ cannot become negative. Because the displacements of the $y'_i$ are the same as the displacements of the $y_i$ (for given realizations of the noise), the mean velocity $v(\rho,\sigma)$ of one particle in the original system must be the same as the mean velocity $v(\rho',\sigma')$ in the transformed system:

$$v(\rho,\sigma) = v(\rho',\sigma') = v\left(\frac{\rho}{1-m\rho}, \sigma - m\lambda\right)\,, \quad m = \text{int}(\sigma/\lambda)\,. \tag{S27}$$

The currents in the two systems are given by $j(\rho,\sigma) = (N/L)v(\rho,\sigma) = \rho\, v(\rho,\sigma)/\lambda$ and $j(\rho',\sigma') = (N/L')v(\rho',\sigma') = \rho' v(\rho',\sigma')/\lambda$. Using Eq. (S27), this yields Eq. (2):

$$j(\rho,\sigma) = \frac{\rho}{\rho'}\, j(\rho',\sigma') = (1 - m\rho)\, j\left(\frac{\rho}{1-m\rho}, \sigma - m\lambda\right)\,, \quad m = \text{int}(\sigma/\lambda)\,. \tag{S28}$$

For $\sigma = m\lambda$ it follows

$$j(\rho, m\lambda) = (1 - m\rho)\, j\left(\frac{\rho}{1 - m\rho}, 0\right) = (1 - m\rho)\, j_0\left(\frac{\rho}{1 - m\rho}\right) = (1 - m\rho)\, \mu f \frac{\rho}{1 - m\rho} = \mu f \rho = j_0(\rho)\,, \qquad \text{(S29)}$$

i.e. the current for commensurable diameters equals the current for non-interacting particles for all $\rho$.

In the range of $\sigma'$ with ASEP-like current-density relation [$\sigma'$ around 0.75, see Fig. 2(a)], it holds $j(\rho, \sigma) \simeq j_{\text{ASEP}}(\rho, \sigma) = (v_0/\lambda)\rho(1 - \rho)$. In that $\sigma'$-range the BASEP corresponds to a monomer ASEP, i.e. an $l$-ASEP with $l$mers of size $l = 1$. Accordingly, $m = \text{int}(\sigma'/\lambda) = 0$ refers to $l = 1$. When considering $\sigma = \sigma' + m\lambda$ with $\sigma'$ in the respective range, one may expect to find a current-density relation corresponding to an $l$-ASEP consisting of $l$mers with $l = m + 1$. Indeed, this follows from Eq. (2):

$$\begin{aligned} j_{\text{ASEP}}(\rho, \sigma) &= (1 - m\rho)\, j_{\text{ASEP}}\left(\frac{\rho}{1 - m\rho}, \sigma - m\lambda\right) = \frac{v_0}{\lambda}\, \rho\left(1 - \frac{\rho}{1 - m\rho}\right) = \frac{v_0}{\lambda}\, \rho \frac{1 - (m+1)\rho}{1 - m\rho} \\ &= \frac{v_0}{\lambda}\, \rho\, \frac{1 - l\rho}{1 - (l-1)\rho} = j_{l-\text{ASEP}}(\rho)\,. \end{aligned} \qquad \text{(S30)}$$

Here, $j_{l-\text{ASEP}}(\rho) = (v/\lambda)\rho[1 - l\rho)/(1 - (l - 1)\rho]$ is the current-density relation of the $l$-ASEP [8], where the prefactor $(v_0/\lambda)$ corresponds to the difference $(\Gamma_+ - \Gamma_-)$ of the hopping rates $\Gamma_+$ and $\Gamma_-$ in and against the bias direction of this lattice model, respectively.

## 5. Examples for NESS phases in the open BASEP

To demonstrate the occurrence of the predicted NESS phases in an open BASEP coupled to two particle reservoirs L and R at its left and right boundary, we performed Monte-Carlo simulations for particles with size $\sigma = 0.62$ and systems with up to $M = 400$ potential wells ($L = 400\,\lambda$). Particles are injected from and ejected to the reservoir L with rates $\Gamma_{\text{in}}^{\text{L}}$ and $\Gamma_{\text{out}}^{\text{L}}$. Likewise, $\Gamma_{\text{in}}^{\text{R}}$ and $\Gamma_{\text{out}}^{\text{R}}$ are the injection and ejection rates for the reservoir R. Particles can only be injected (ejected) if the last well at the boundaries is empty (occupied). The rates are parameterized by two variables $\gamma_{\text{L}}$ and $\gamma_{\text{R}}$ of order one. Specifically, we set $\Gamma_{\text{in}}^{\text{L}} = \gamma_{\text{L}}\Gamma_0$, $\Gamma_{\text{out}}^{\text{L}} = \Gamma_{\text{in}}^{\text{L}} \exp(-\beta f\lambda)$, $\Gamma_{\text{out}}^{\text{R}} = \gamma_{\text{R}}\Gamma_0$, and $\Gamma_{\text{in}}^{\text{R}} = \Gamma_{\text{out}}^{\text{R}} \exp(-\beta f\lambda)$, where $\Gamma_0$ is the mean rate of a single particle to move from well to a neighboring one [9].

Figure S2 shows profiles of the period-averaged densities $\bar{\rho}_i$, $i = 1, \ldots, M$, in this open BASEP for $\beta f\lambda = f = 1$ and different values of $\gamma_{\text{L}}$ and $\gamma_{\text{R}}$. These profiles exemplify different phases predicted by the phase diagram in Fig. 4(a). In Figs. S2(c), we indicated by the dashed line the density $\rho_{\max}$, i.e. where $j(\rho, \sigma = 0.62)$ attains its maximum in Fig. 2(a).

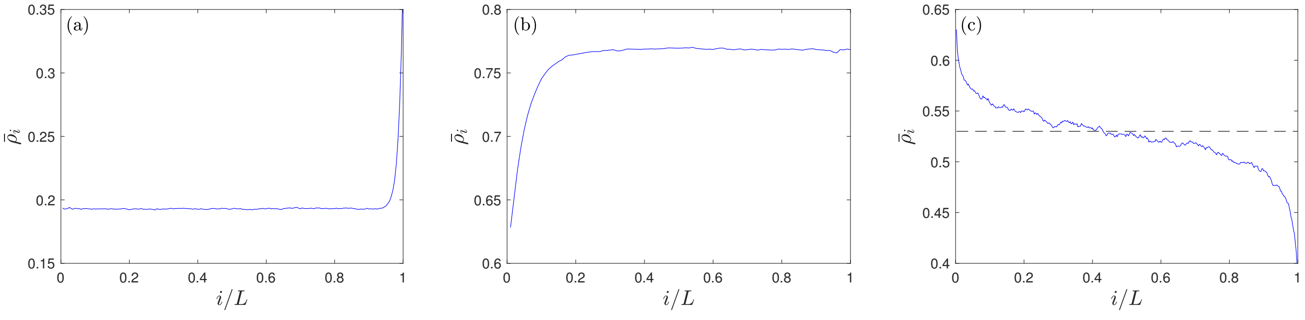


FIG. S2. Demonstration of different NESS phases in an open BASEP with particles of size $\sigma = 0.62$. The BASEP is coupled to two reservoirs L and R at its left and right boundary, where injection and ejection rates are parameterized by $\gamma_{\text{L}}$ and $\gamma_{\text{R}}$ (see text). The profiles of the period-averaged densities $\bar{\rho}_i$ demonstrate the occurrence of (a) a left-boundary induced phase for $(\gamma_{\text{L}}, \gamma_{\text{R}}) = (0.1, 0.5)$ with $\rho_{\text{b}} = \rho_{\text{L}} \cong 0.19$, (b) a right-boundary induced phase for $(\gamma_{\text{L}}, \gamma_{\text{R}}) = (0.7, 0.15)$ with $\rho_{\text{b}} = \rho_{\text{R}} \cong 0.77$, and (c) a maximal current phase for $(\gamma_{\text{L}}, \gamma_{\text{R}}) = (0.9, 0.8)$ with $\rho_{\text{b}} = \rho_{\max} \cong 0.53$. In (c) the bulk density is indicated by the dashed line.

[1] V. Ambegaokar and B. I. Halperin, Phys. Rev. Lett. **22**, 1364 (1969).
[2] J. K. Percus, J. Stat. Phys. **15**, 505 (1976).
[3] A. R. Bishop, W. Dieterich, and I. Peschel, Z. Phys. B **33**, 187 (1979).
[4] W. Dieterich, P. Fulde, and I. Peschel, Adv. Phys. **29**, 527 (1980).
[5] U. M. B. Marconi and P. Tarazona, J. Chem. Phys. **110**, 8032 (1999).
[6] H. Löwen and M. Heinen, Eur. Phys. J. Special Topics **223**, 3113 (2014).
[7] D. Lips, A. Ryabov, and P. Maass, to be published.
[8] G. Lakatos and T. Chou, J. Phys. A: Math. Gen. **36**, 2027 (2003).
[9] L. Dagdug and A. M. Berezhkovskii, J. Chem. Phys. **131**, 056101 (2009).
